# Supplementary material for: Deep Evaluation Metric: Learning to Evaluate Simulated Radar Point Clouds for Virtual Testing of Autonomous Driving
Source: arXiv:2104.06772 source file (2021-06-21)
Supplement: Supplementary file 1 [file 06_appendix.tex]

\section*{APPENDIX}
\label{appendix}
